# Supplementary material for: Improving Function Coverage with Munch: A Hybrid Fuzzing and Directed Symbolic Execution Approach
Source: arXiv:1711.09362 source file (2017-12-12)
Supplement: Supplementary file 1 [file appendix-coverage-stats.tex]

\vspace{4em}
\section{Coverage statistics}\label{sec:coverage-statistics}

\begin{table}[h!]
    \centering
    \caption{Call-graph-depth-wise function coverage for \emph{Bc}}
    \label{tab:bciff-depth-coverage}
    \begin{tabular}{@{} c c c c@{}}
        \toprule
        Depth & KLEE (\%) & AFL (\%) & Hybrid (\%) \\ \midrule
        0 & 100 & 100 & 100 \\
        1 & 100 & 100 & 100 \\
        2 & 46  & 63  & 79  \\
        3 & 26  & 63  & 74  \\
        4 & 5   & 43  & 45  \\
        5 & 6   & 22  & 22  \\
        6 & 0   & 0   & 0 \\ \bottomrule
    \end{tabular}
\end{table}

\begin{table}[h!]
    \centering
    \caption{Call-graph-depth-wise function coverage for \emph{Bzip2}}
    \label{tab:bzip2-depth-coverage}
   \begin{tabular}{@{} c c c c@{}}
        \toprule
        Depth & KLEE (\%) & AFL (\%) & Hybrid (\%) \\ \midrule
        0  & 100 & 100 & 100 \\
        1  & 90  & 50  & 80  \\
        2  & 50  & 61  & 61  \\
        3  & 17  & 28  & 28  \\
        4  & 40  & 30  & 30  \\
        5  & 25  & 63  & 63  \\
        6  & 0   & 50  & 50  \\
        7  & 0   & 100 & 100 \\
        8  & 0   & 80  & 80  \\
        9  & 0   & 50  & 50  \\
        10 & 0   & 33  & 33  \\
        11 & 0   & 0   & 0 \\ \bottomrule
    \end{tabular}
\end{table}

\begin{table}[h!]
    \centering
    \caption{Call-graph-depth-wise function coverage for \emph{Diff}}
    \label{tab:diff-depth-coverage}
   \begin{tabular}{@{} c c c c@{}}
        \toprule
        Depth & KLEE (\%) & AFL (\%) & Hybrid (\%) \\ \midrule
       0  & 100 & 100 & 100 \\
       1  & 60  & 48  & 64  \\
       2  & 39  & 25  & 36  \\
       3  & 27  & 62  & 70  \\
       4  & 23  & 30  & 40  \\
       5  & 0   & 38  & 38  \\
       6  & 0   & 31  & 31  \\
       7  & 0   & 25  & 25  \\
       8  & 0   & 0   & 0   \\
       9  & 0   & 0   & 0   \\
       10 & 0   & 0   & 0   \\
       11 & 0   & 0   & 0   \\
       12 & 0   & 0   & 0   \\
       13 & 0   & 0   & 0 \\ \bottomrule
    \end{tabular}
\end{table}

\begin{table}[h!]
    \centering
    \caption{Call-graph-depth-wise function coverage for \emph{Grep}}
    \label{tab:grep-depth-coverage}
    \begin{tabular}{@{} c c c c@{}}
        \toprule
        Depth & KLEE (\%) & AFL (\%) & Hybrid (\%) \\ \midrule
0 & 100 & 100 & 100 \\
1 & 66  & 31  & 45  \\
2 & 38  & 8   & 15  \\
3 & 14  & 21  & 24  \\
4 & 12  & 8   & 10  \\
5 & 11  & 0   & 0   \\
6 & 0   & 0   & 0   \\
7 & 0   & 0   & 0   \\
8 & 0   & 0   & 0   \\ \bottomrule
    \end{tabular}
\end{table}

\begin{table}[h!]
    \centering
    \caption{Call-graph-depth-wise function coverage for \emph{Sed}}
    \label{tab:sed-depth-coverage}
    \begin{tabular}{@{} c c c c@{}}
        \toprule
        Depth & KLEE (\%) & AFL (\%) & Hybrid (\%) \\ \midrule
0  & 100 & 100 & 100 \\
1  & 100 & 67  & 83  \\
2  & 100 & 69  & 81  \\
3  & 87  & 54  & 72  \\
4  & 44  & 32  & 40  \\
5  & 55  & 9   & 9   \\
6  & 57  & 0   & 0   \\
7  & 0   & 0   & 0   \\
8  & 0   & 0   & 0   \\
9  & 0   & 0   & 0   \\
10 & 0   & 0   & 0   \\
11 & 0   & 0   & 0 \\ \bottomrule
    \end{tabular}
\end{table}

\clearpage
\begin{minipage}{\linewidth}
\vspace{-3.3em}
\begin{table}[H]
    \centering
    \caption{Call-graph-depth-wise function coverage for \emph{Flex}}
    \label{tab:flex-depth-coverage}
    \begin{tabular}{@{} c c c c@{}}
        \toprule
        Depth & KLEE (\%) & AFL (\%) & Hybrid (\%) \\ \midrule
         0 & 100 & 100 & 100 \\
         1 & 100 & 100 & 100 \\
         2 & 43  & 100 & 100 \\
         3 & 19  & 71  & 71  \\
         4 & 14  & 65  & 67  \\
         5 & 13  & 58  & 58  \\
         6 & 67  & 67  & 67 \\ \bottomrule
    \end{tabular}
\end{table}

\begin{table}[H]
    \centering
    \caption{Call-graph-depth-wise function coverage for \emph{jq}}
    \label{tab:jq-depth-coverage}
    \begin{tabular}{@{} c c c c@{}}
        \toprule
        Depth & KLEE (\%) & AFL (\%) & Hybrid (\%) \\ \midrule
         0 & 100 & 100 & 100 \\
         1 & 64  & 85  & 97  \\
         2 & 58  & 85  & 87  \\
         3 & 35  & 73  & 73  \\
         4 & 32  & 70  & 70  \\
         5 & 11  & 71  & 71  \\
         6 & 12  & 73  & 73  \\
         7 & 54  & 69  & 69  \\
         8 & 0   & 0   & 0   \\
         9 & 0   & 0   & 0 \\ \bottomrule
    \end{tabular}
\end{table}

\begin{table}[H]
    \centering
    \caption{Call-graph-depth-wise function coverage for \emph{Lz4}}
    \label{tab:lz4-depth-coverage}
    \begin{tabular}{@{} c c c c@{}}
        \toprule
        Depth & KLEE (\%) & AFL (\%) & Hybrid (\%) \\ \midrule
         0 & 100 & 100 & 100 \\
         1 & 100 & 19  & 71  \\
         2 & 71  & 18  & 59  \\
         3 & 65  & 40  & 75  \\
         4 & 67  & 29  & 58  \\
         5 & 43  & 0   & 43  \\
         6 & 67  & 0   & 67  \\
         7 & 0   & 0   & 0 \\ \bottomrule
    \end{tabular}
\end{table}

\begin{table}[H]
    \centering
    \caption{Call-graph-depth-wise function coverage for \emph{Zopfli}}
    \label{tab:zopfli-depth-coverage}
   \begin{tabular}{@{} c c c c@{}}
        \toprule
        Depth & KLEE (\%) & AFL (\%) & Hybrid (\%) \\ \midrule
         0  & 100 & 100 & 100 \\
         1  & 100 & 100 & 100 \\
         2  & 67  & 100 & 100 \\
         3  & 67  & 67  & 67  \\
         4  & 67  & 67  & 67  \\
         5  & 50  & 75  & 75  \\
         6  & 21  & 79  & 79  \\
         7  & 4   & 92  & 92  \\
         8  & 4   & 100 & 100 \\
         9  & 0   & 100 & 100 \\
         10 & 0   & 100 & 100 \\
         11 & 0   & 100 & 100 \\ \bottomrule
    \end{tabular}
\end{table}

\end{minipage}%
\begin{minipage}{0.06\linewidth}%
\color{white}{.}
\end{minipage}%
