# Supplementary material for: Improving Function Coverage with Munch: A Hybrid Fuzzing and Directed Symbolic Execution Approach
Source: arXiv:1711.09362 source file (2017-12-12)
Supplement: Supplementary file 3 [file appendix-generated-program.tex]

\begin{minipage}{0.86\linewidth}
\vspace{1.5em}%
\section{Artificially generated program}\label{sec:appendix-artifical-programs}
\lstinputlisting[label=list:artificial-program, language=C, caption=An artificially generated program with branching factor of 2 and call-graph depth of 3.,firstline=4, firstnumber=4]{code/level3.c}
\end{minipage}
