# Supplementary material for: Improving Function Coverage with Munch: A Hybrid Fuzzing and Directed Symbolic Execution Approach
Source: arXiv:1711.09362 source file (2017-12-12)
Supplement: Supplementary file 4 [file appendix-klee-command.tex]

\section{KLEE command for targeted search}\label{sec:klee-command}
\begin{minipage}{0.87\linewidth}
\begin{lstlisting}[label=list:targeted-search-command, caption=Example KLEE targeted-search command.]
klee --posix-runtime --libc=uclibc \
--only-output-states-covering-new \
--disable-inlining \
-output-dir=~/klee-out-mbsstr \
-optimize --max-time=300 \
-max-solver-time=15 --watchdog \
-search=sonar\
-sonar-target=function-call\
-sonar-target-info=mbsstr diff.x.bc \
-sym-args 1 2 50 -sym-files 1 100
\end{lstlisting}
\end{minipage}
